# Supplementary material for: Solving Forward and Inverse Problems of Contact Mechanics using Physics-Informed Neural Networks
Source: arXiv:2308.12716 source file (2023-08-24)
Supplement: Supplementary file 1 [file gn.tex]

\section{Calculation of the gap}\label{append_gn}
%To enforce KKT constraints, a gap in the normal direction has to be calculated. 
In the following sections, we focus on two-dimensional contact problems between an elastic $\Omega^{(e)}$ and a rigid flat domain $\Omega^{(r)}$ 
as illustrated in Fig. \ref{fig:gap_function}. The gap $g_n$ refers to 
the projected distance from the elastic domain on the rigid flat domain in the normal direction. 
Using geometrical similarity we can obtain the following relation

\begin{equation}
    \label{eq:gap}
    \frac{g_n}{g_{n_y}} = \frac{ \lVert \boldsymbol{n}\rVert}{|n_y|_{abs}},
\end{equation}

\afterequation
Here, $||.||$ denotes the norm of a vector and $|.|_{abs}$ refers to the absolute value. Since $\boldsymbol{n}$
is a unit vector, $\lVert \boldsymbol{n}\rVert$=1. The projection of gap in the y direction $g_{n_y}$ on the rigid domain 
can be determined as (see Eq. \ref{eq:displacementvector})

\begin{equation}
    \label{eq:gapy}
    g_{n_y} = Y + u_y, 
\end{equation}

\afterequation
where $Y$ is the y coordinate in the reference configuration and $u_y$ is the y component of the displacement field.
Inserting Eq. \ref{eq:gapy} into Eq. \ref{eq:gap} leads to 

\begin{equation}
    \label{eq:gapfinal}
    {g_n} = \frac{Y + u_y}{|n_y|_{abs}}.
\end{equation}

\begin{figure}[thbp]
    \centering
    \includegraphics[width=0.55\linewidth]{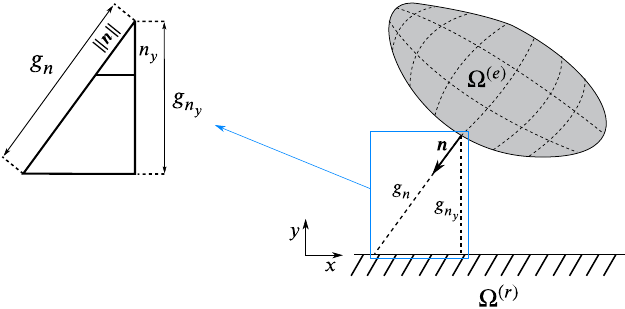}  
    \caption{An illustration of the relation between the gap in the normal direction $g_n$ and the gap in the y direction $g_y$.}
    \label{fig:gap_function}
\end{figure}

The term $|n_y|_{abs}$ is in the denominator (see Eq. \ref{eq:gapfinal}), so it can not be zero, which requires well-defined boundary normals. 
For instance, complex shapes can contain sharp edges that can have the zero-valued
boundary normal component $n_y$. Thus, special treatment for sharp edges is required. 
Note that the way we calculate the gap is one of the simplest methods and it may not be generalized for complex problems. 
Since the PINN formulation for contact mechanics is based on linear elasticity and we will consider 
only benchmark problems in the next sections, the gap formulation is sufficient. 
For further reading, we refer to \cite{popp2012mortar} \cite{popp2009finite}.
