# Supplementary material for: Solving Forward and Inverse Problems of Contact Mechanics using Physics-Informed Neural Networks
Source: arXiv:2308.12716 source file (2023-08-24)
Supplement: Supplementary file 2 [file mesh.tex]

\section{Distributions of test points}\label{append_mesh}
Fig. \ref{fig:meshes} shows distributions of test points to evaluate errors for each numerical example. 
For each numerical example, structured meshes are used to generate collocation and boundary points. 

\begin{figure}[thbp]
    \def\figsize{0.325}
    \def\hskiplocal{\hskip 0cm}
    \centering
    \begin{tabular}{c@{\hskiplocal}c@{\hskiplocal}c}
        \includegraphics[trim={25cm 5cm 25cm 5cm},clip,width=\figsize\linewidth]{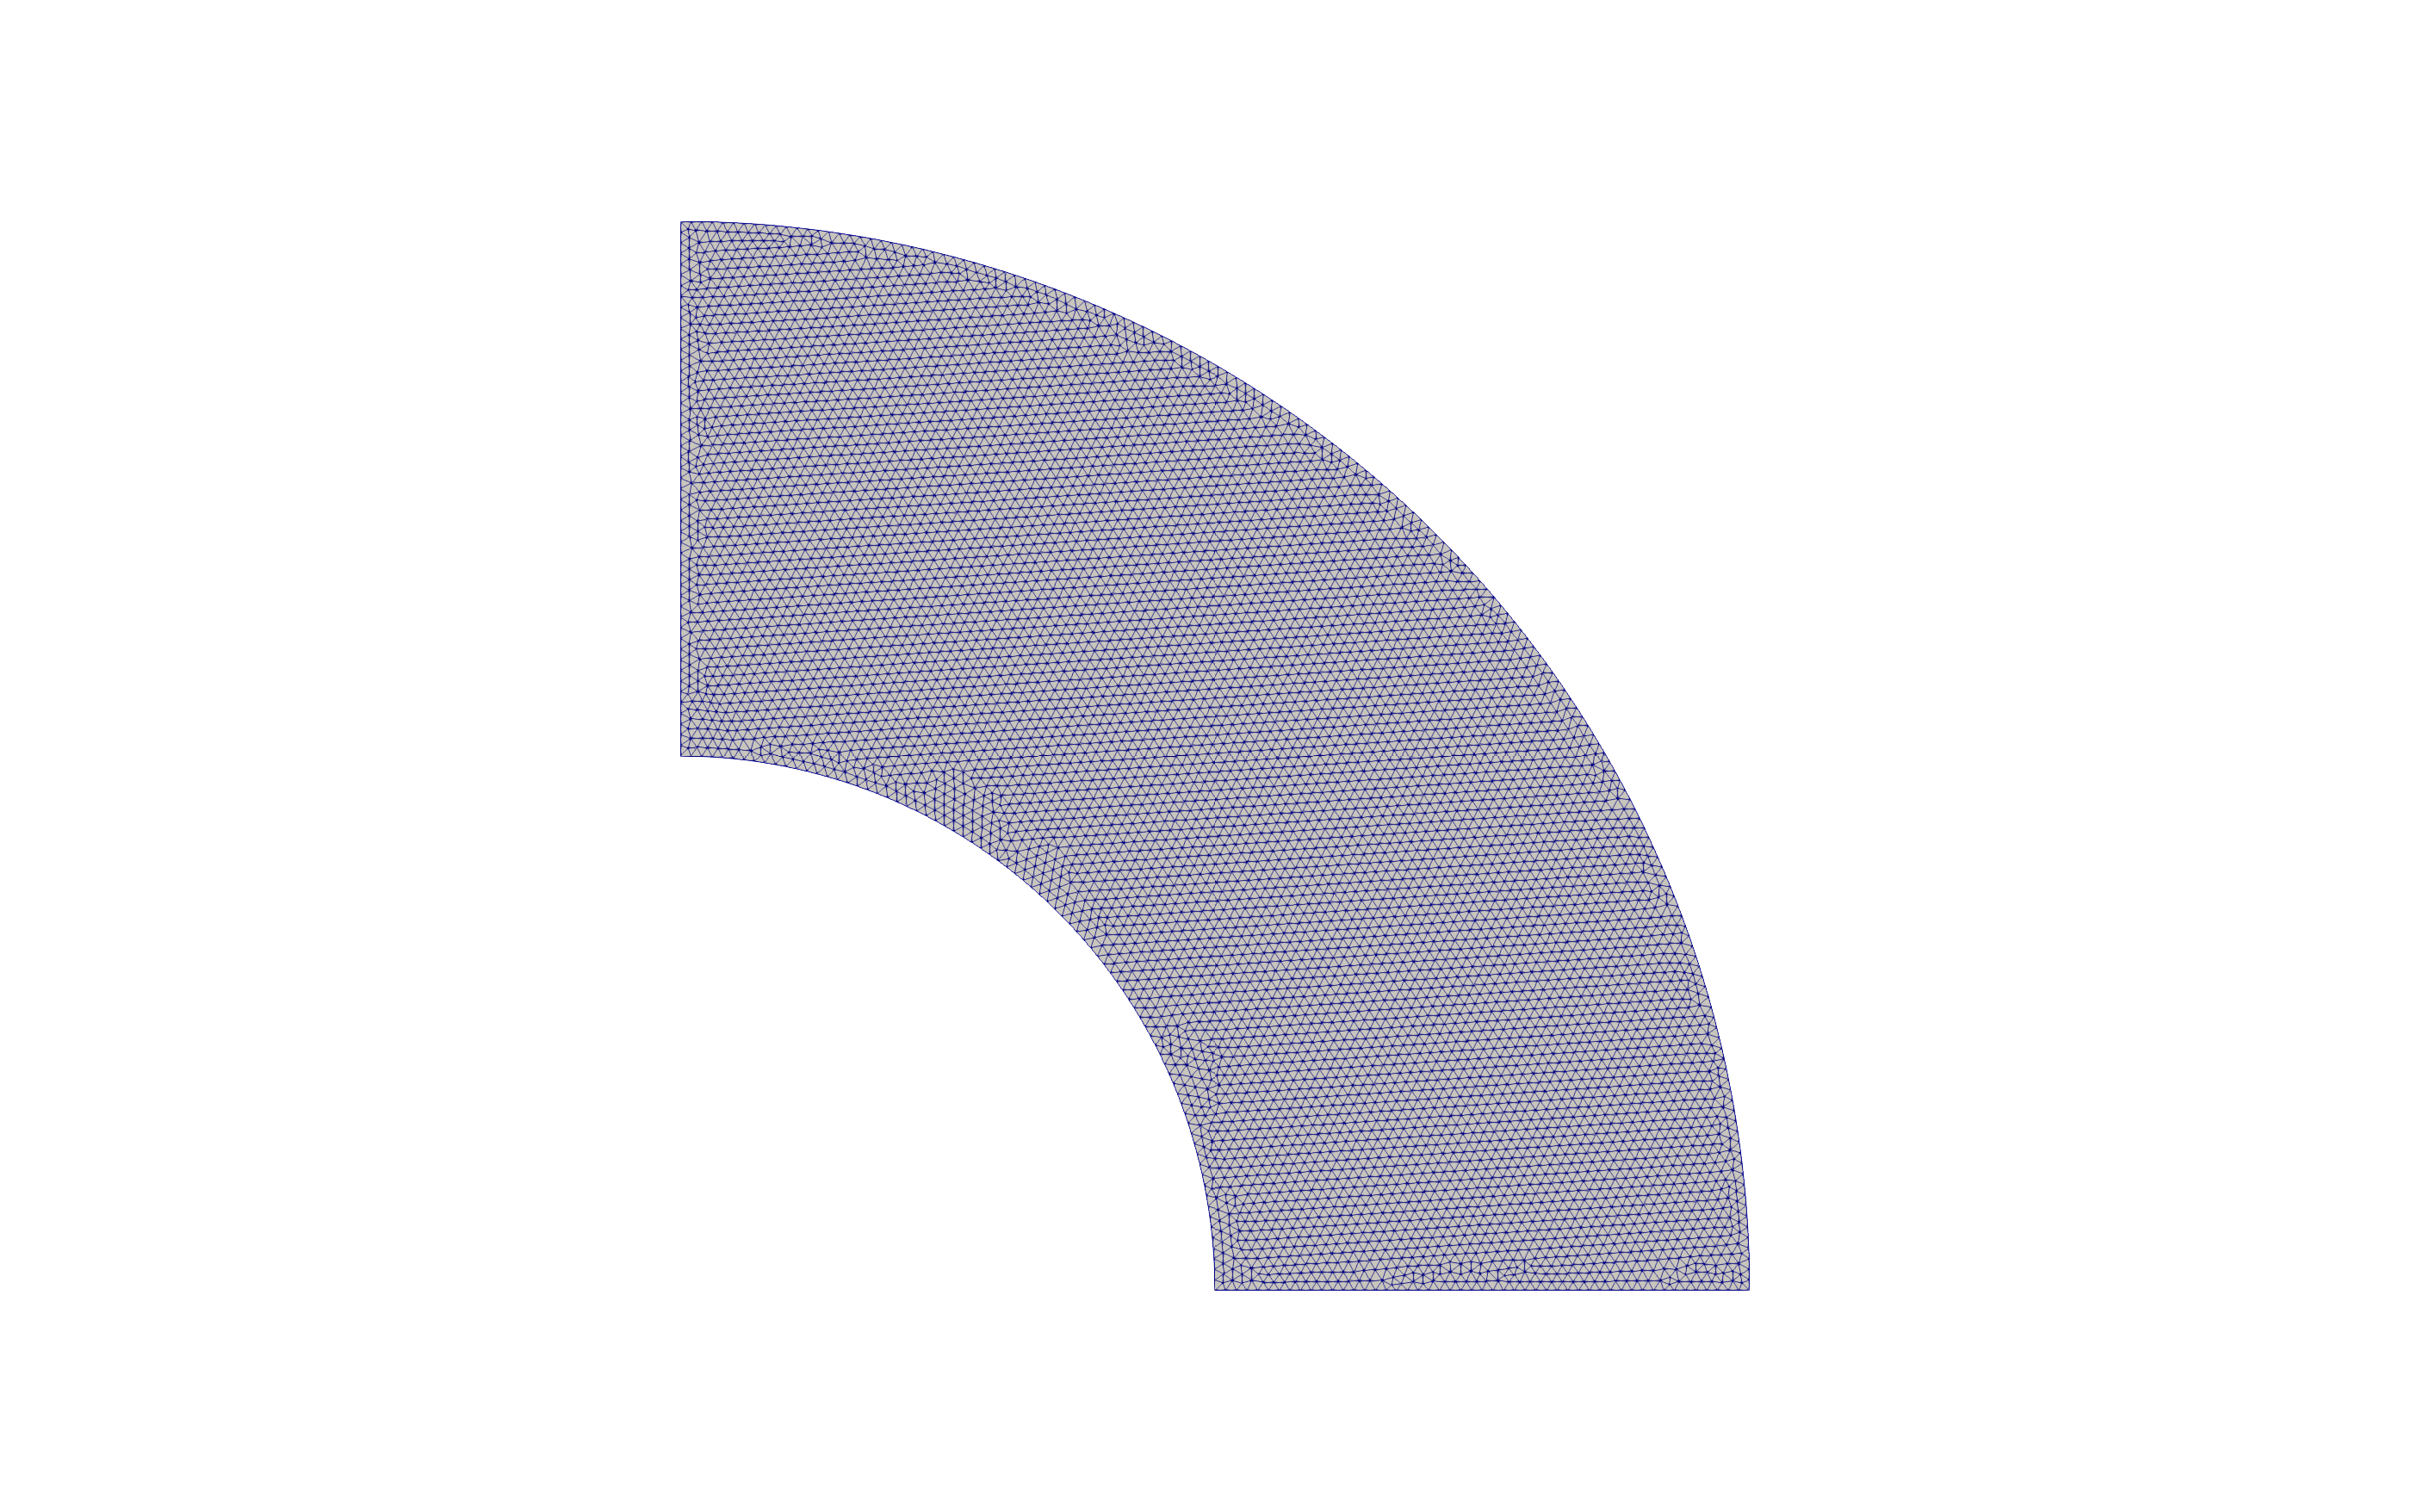}&
        \includegraphics[trim={25cm 5cm 25cm 5cm},clip,width=\figsize\linewidth]{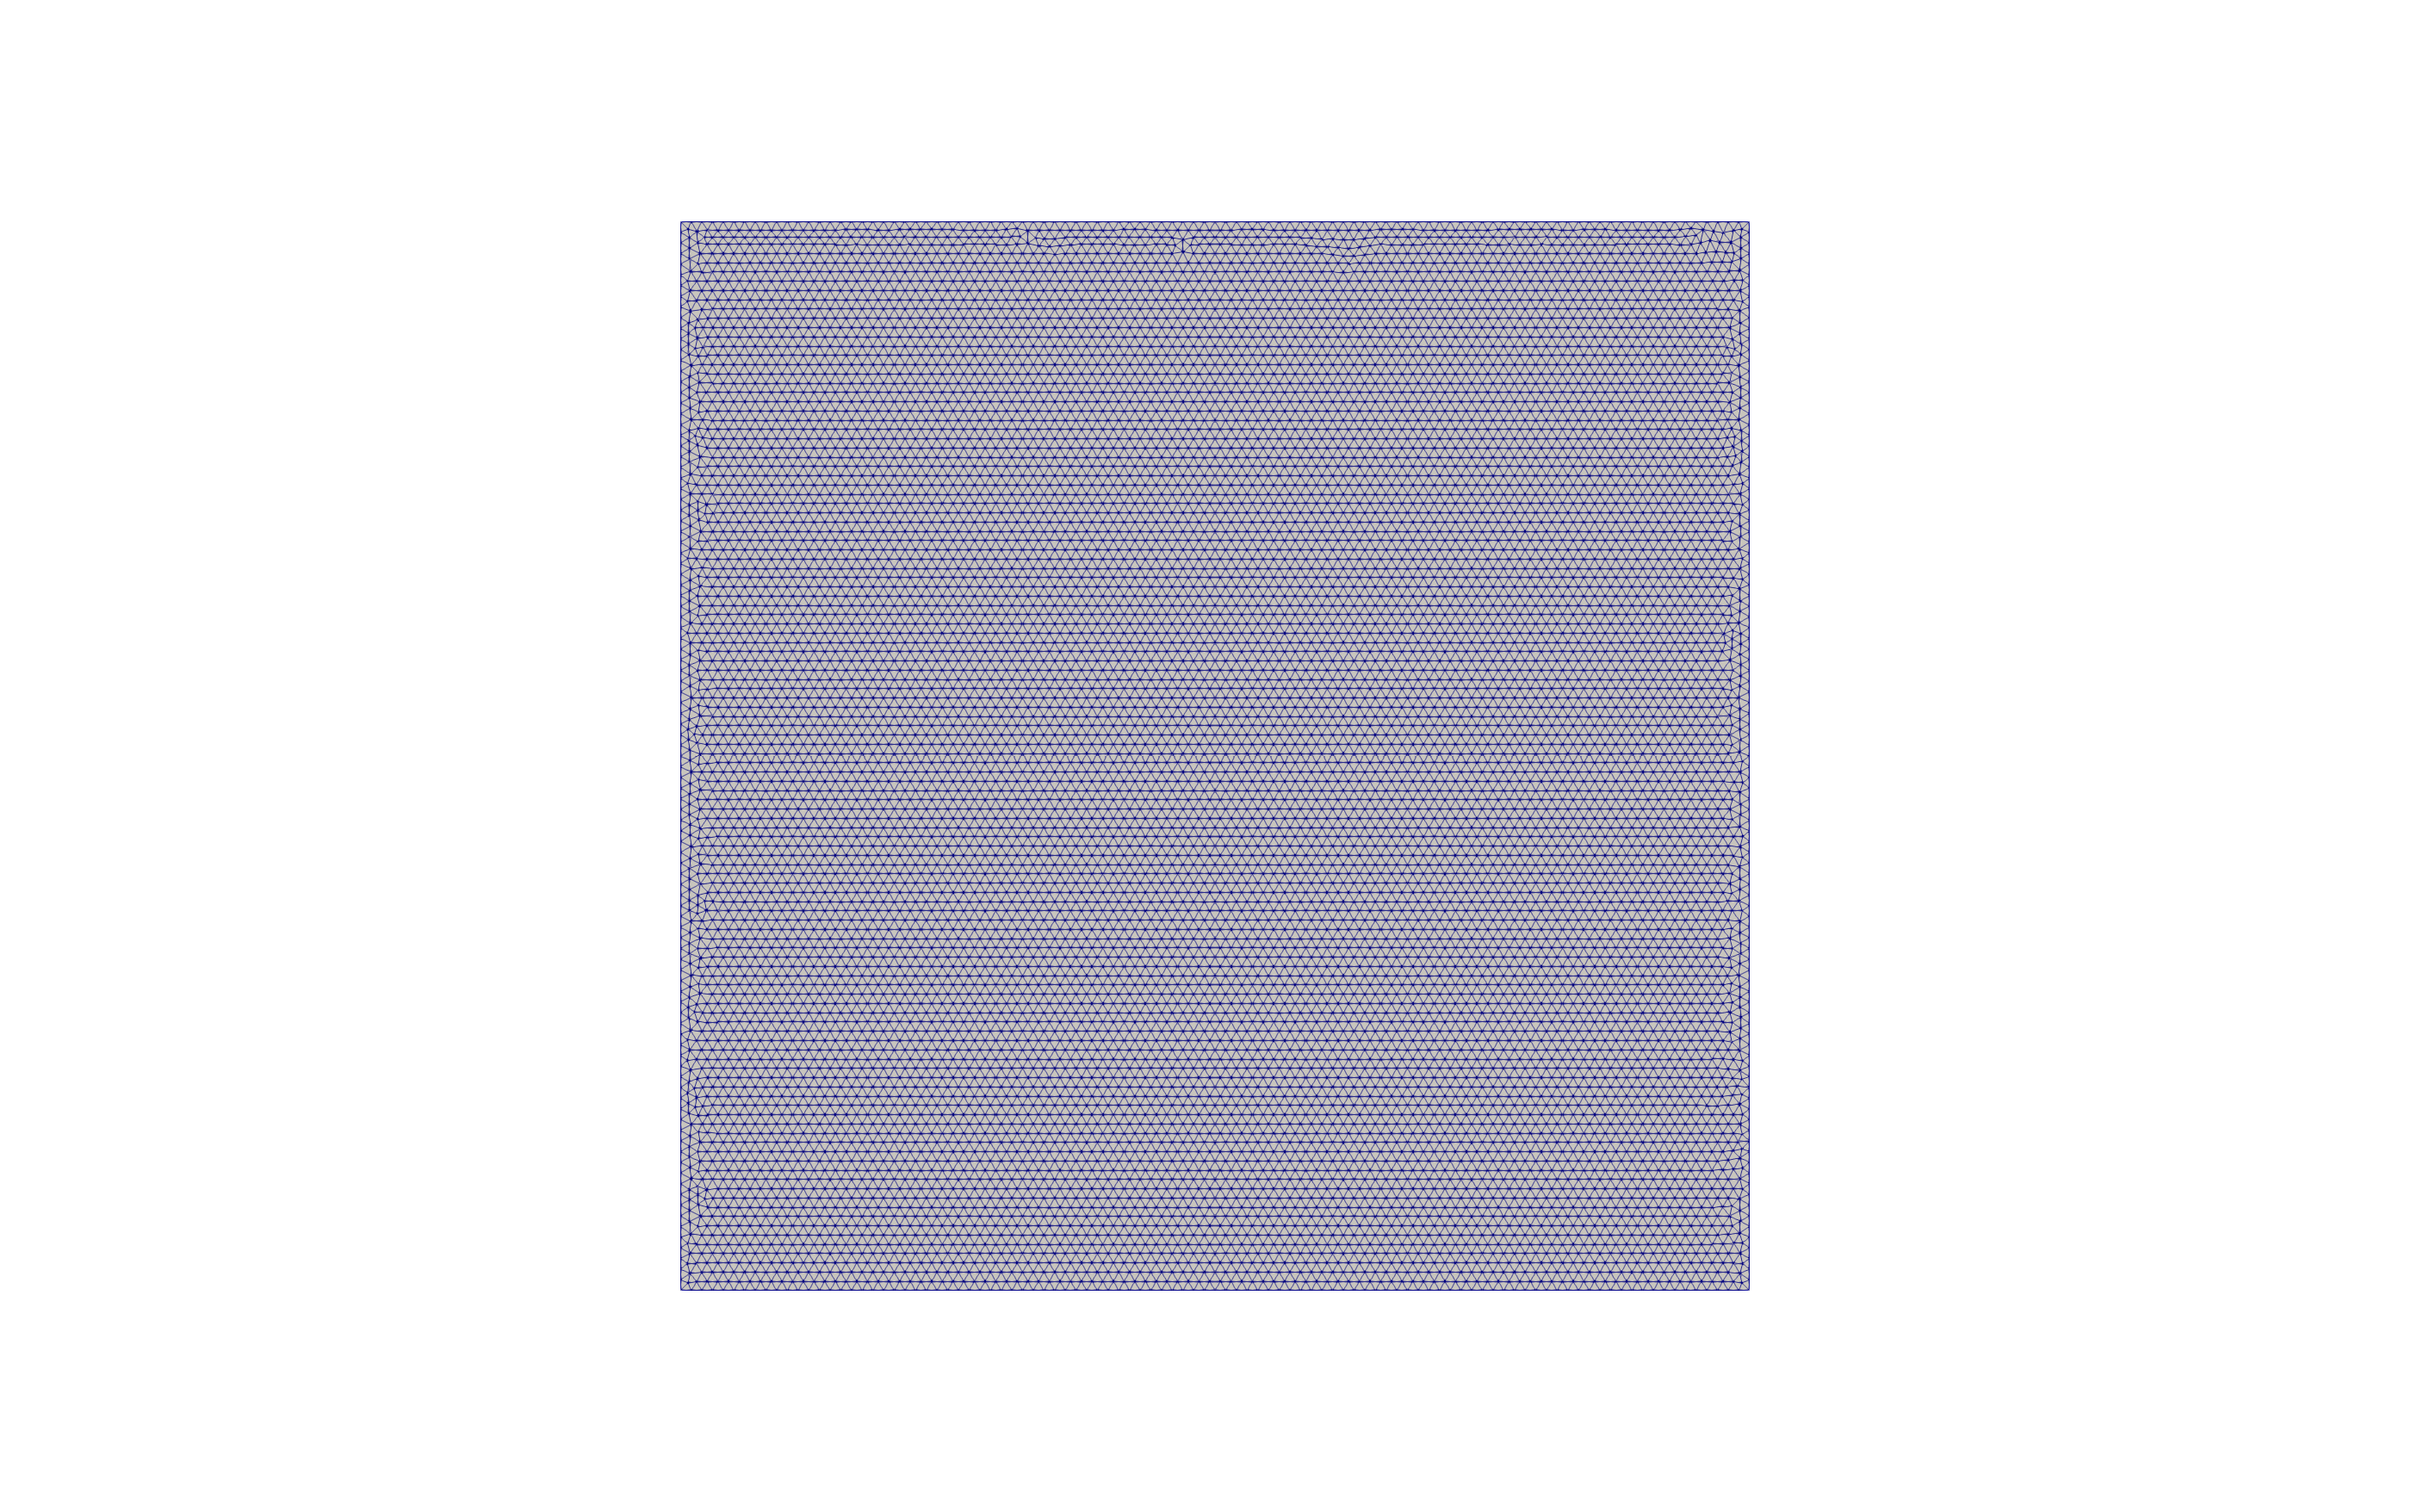}&
        \includegraphics[trim={25cm 5cm 25cm 5cm},clip,width=\figsize\linewidth]{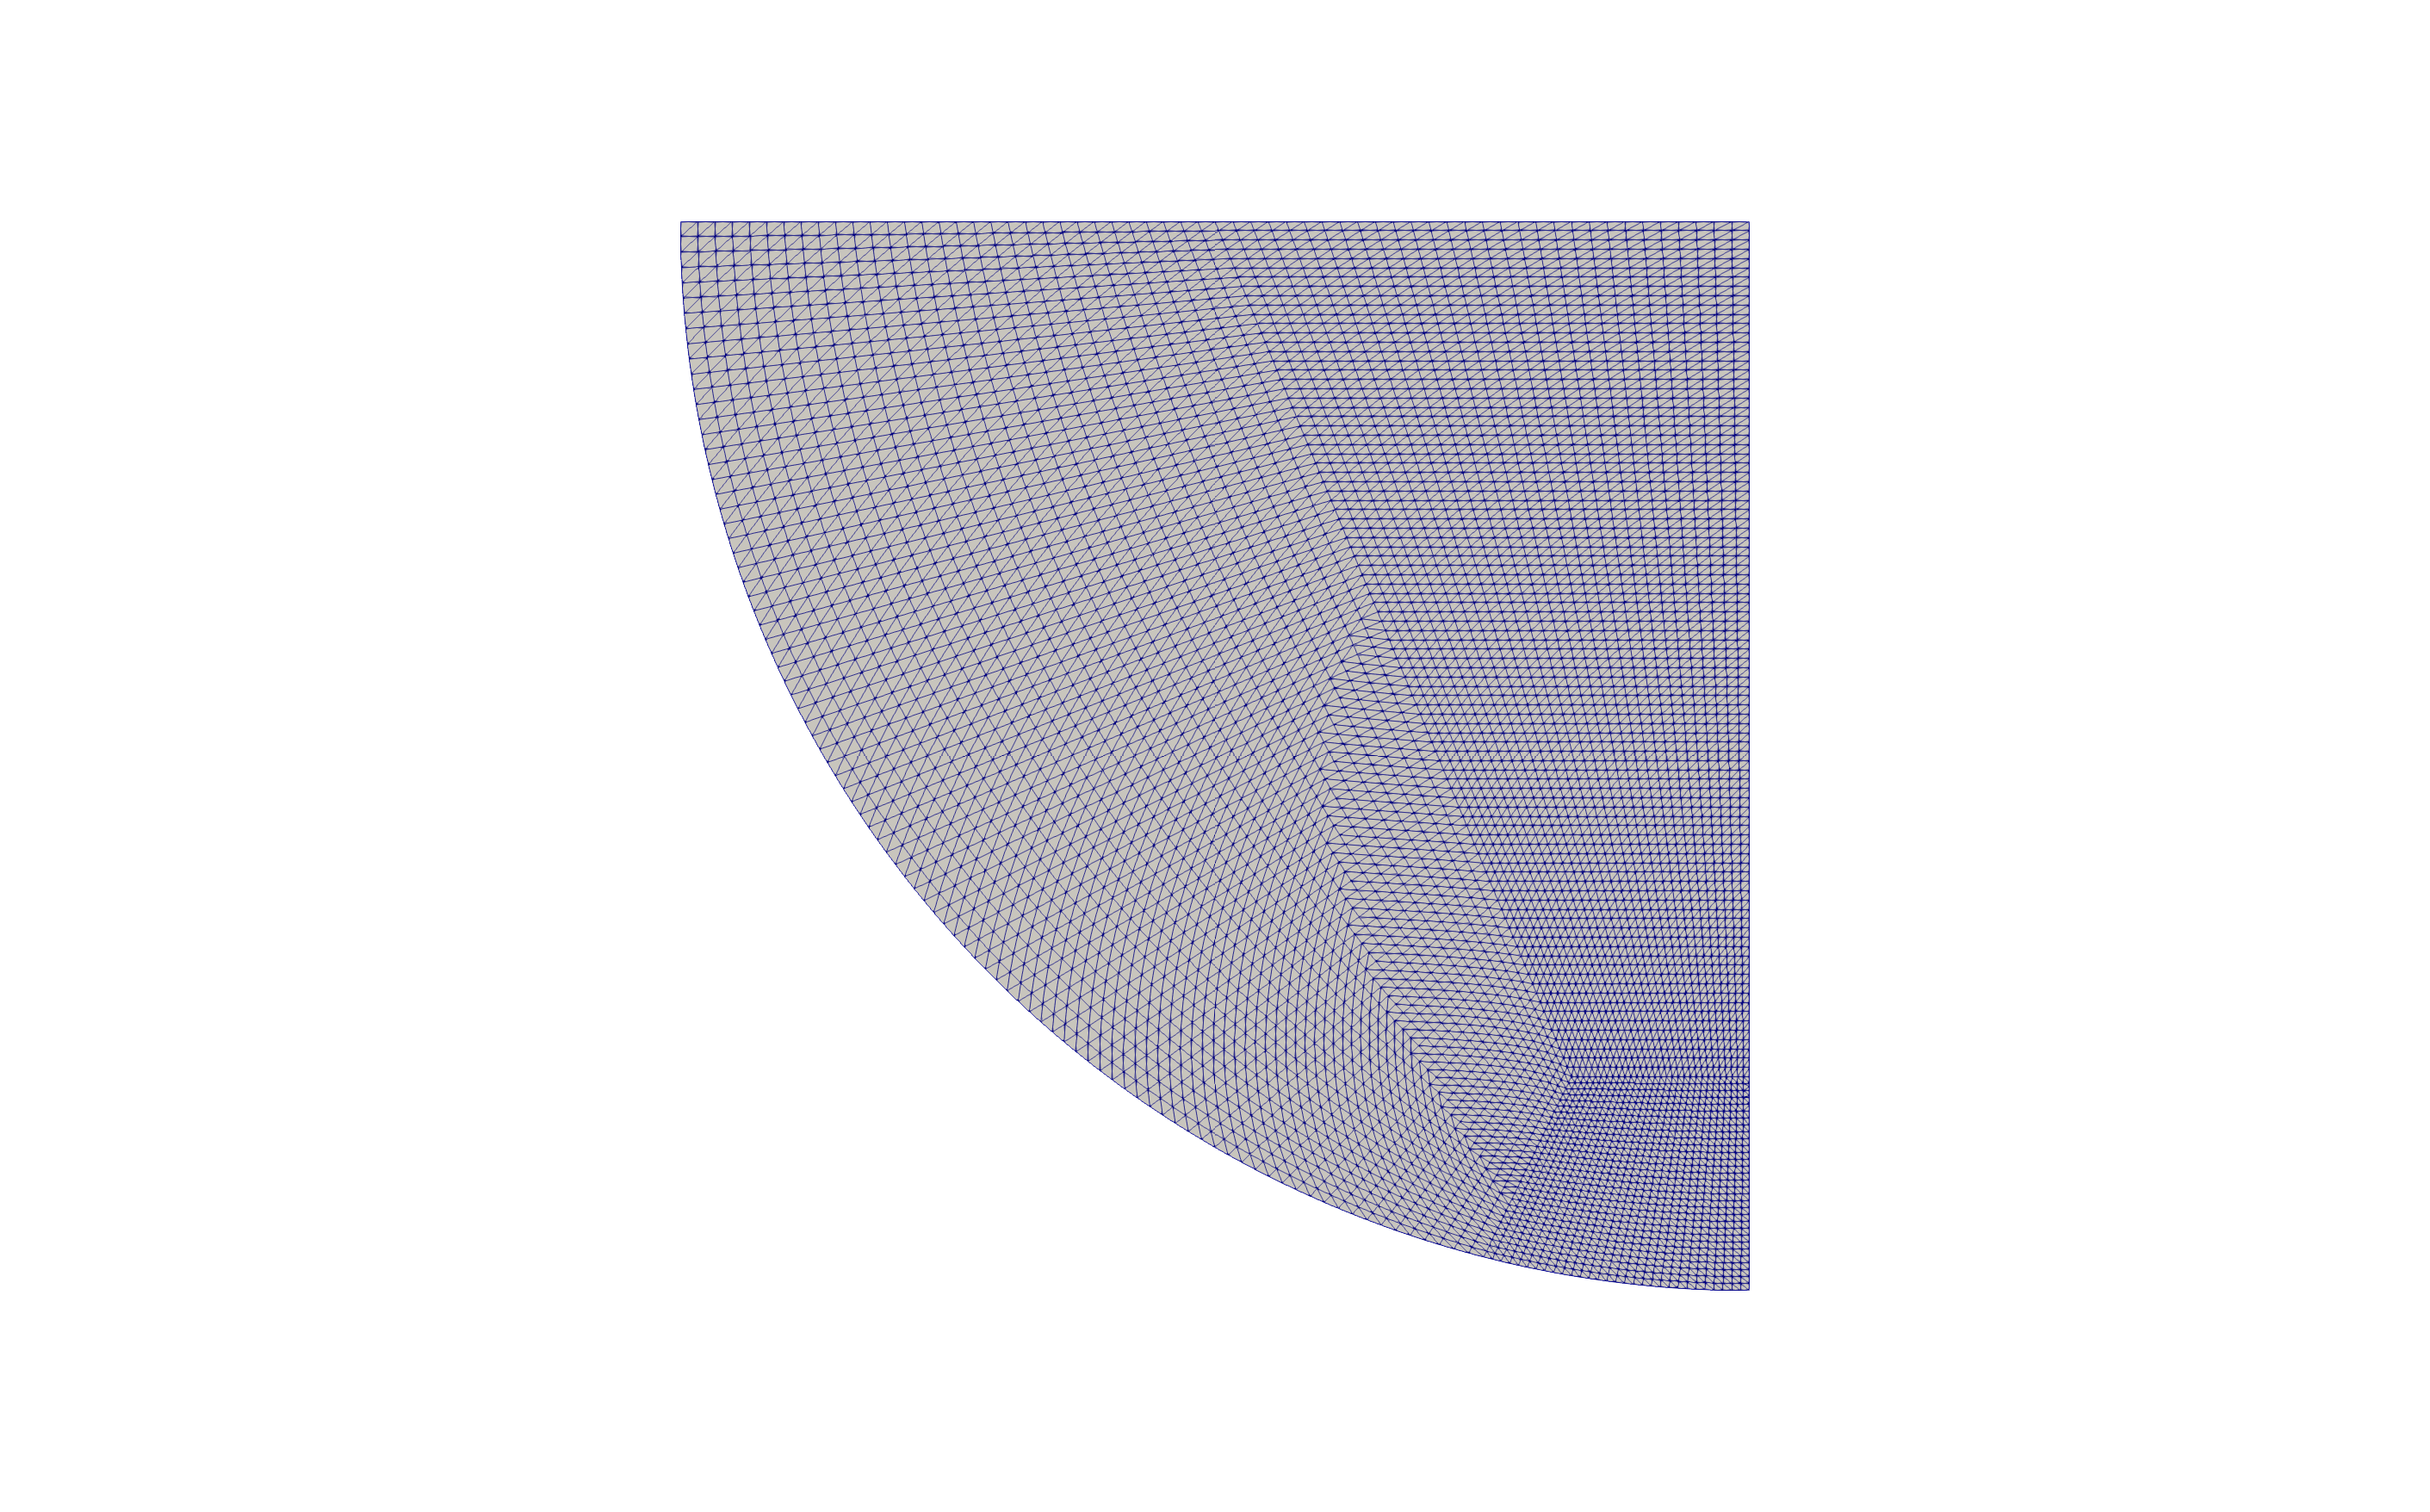}\\
        (a) & (b) & (c)
    \end{tabular}
    \caption{Meshes for numerical examples.} %
    \label{fig:meshes}
\end{figure}
